# Supplementary material for: Classification robustness to common optical aberrations
Source: arXiv:2308.15499 source file (2023-08-29)
Supplement: Supplementary file 1 [file supp_additional.tex]

%%%%%%%%%%%%%%%%%%%%% deprecated %%%%%%%%%%%%%%%%%%%%%%%%%%%%%%%%%%%%

\iffalse
\clearpage

\begin{figure}[h]
    \centering
\includegraphics[width=\linewidth]{figures/eval_rg/report_acc_over_severitysplit_corruptions_refvar_alexnet_drefvar_val.pdf}
    \caption{Corruption error metric as from Hendrycks et al. All severities and DNNs. Color groups represent the different corruptions.}
    \label{fig:my_label}
\end{figure}


\begin{figure}[h]
    \centering
    \includegraphics[width=\linewidth]{figures/eval_rg/report_acc_over_severitysplit_corruptions_mode_defocus_blurrefvar_val.pdf}
    \caption{Relative accuracy of defocus blur to clean data. Inset values: Maximum and standard deviation. $100\%$ means equal values.}
    \label{fig:my_label}
\end{figure}

\begin{figure}[h]
    \centering
    \includegraphics[width=\linewidth]{figures/eval_rg/report_acc_over_severitysplit_corruptions_mode_trefoilrefvar_val.pdf}
    \caption{Relative accuracy of trefoil to clean data.}
    \label{fig:my_label}
\end{figure}

\begin{figure}[h]
    \centering
    \includegraphics[width=\linewidth]{figures/eval_rg/report_acc_over_severitysplit_corruptionsrefvar_val.pdf}
    \caption{Relative accuracy of all corruptions to clean data.}
    \label{fig:my_label}
\end{figure}

\begin{figure}[h]
    \centering
    \includegraphics[width=\linewidth]{figures/eval_rg/report_acc_over_severitysplit_corruptionsrefvar_defocus_blur.pdf}
    \caption{Relative accuracy of all corruptions compared to defocus blur (without clean data).}
    \label{fig:my_label}
\end{figure}

\begin{figure}
    \centering \includegraphics[width=\linewidth]{figures/eval_rg/report_acc_over_severitysplit_corruptions_mode_defocus_blurrefvar_alexnet.pdf}
    \caption{Defocus blur (Hendrycks et al.) vs. severity normed to AlexNet acc.}
    \label{fig:my_label}
\end{figure}

\begin{figure}
    \centering \includegraphics[width=\linewidth]{figures/eval_rg/report_acc_over_severitysplit_corruptions_mode_astigmatismrefvar_alexnet.pdf}
    \caption{Astigmatism vs. severity normed to AlexNet acc.}
    \label{fig:my_label}
\end{figure}

\begin{figure}
    \centering \includegraphics[width=\linewidth]{figures/eval_rg/report_acc_over_severitysplit_corruptions_mode_comarefvar_alexnet.pdf}
    \caption{Coma vs. severity normed to AlexNet acc.}
    \label{fig:my_label}
\end{figure}

\clearpage
%
\begin{figure}
    \centering
    \includegraphics[width=\linewidth]{figures/eval_rg/report_acc_over_severitysplit_corruptions_mode_defocus_sphericalrefvar_defocus_blur.pdf}
    \caption{Relative accuracy of spherical and defocus to Hendrycks et al. defocus blur.}
    \label{fig:my_label}
\end{figure}
%
\begin{figure}
    \centering
    \includegraphics[width=\linewidth]{figures/eval_rg/report_acc_over_severitysplit_corruptions_mode_astigmatismrefvar_defocus_blur.pdf}
    \caption{Relative accuracy of astigmatism to defocus blur.}
    \label{fig:my_label}
\end{figure}
%
\begin{figure}
    \centering
    \includegraphics[width=\linewidth]{figures/eval_rg/report_acc_over_severitysplit_corruptions_mode_comarefvar_defocus_blur.pdf}
    \caption{Relative accuracy for coma and defocus blur.}
    \label{fig:my_label}
\end{figure}
%
%%%%%%%%%%%% kernel report (experimental)
%
\begin{figure}[h]
    \centering
    \includegraphics[page=10,width=\linewidth]{figures/matching/report_sheets_final_cooke_rgb.pdf}
    \caption{Geometric defocus blur from Hendrycks et al. vs. PSF defocus blur and chromatic aberration.}
    \label{fig:my_label}
\end{figure}
%
\begin{figure}[h]
    \centering
    \includegraphics[page=19,width=\linewidth]{figures/matching/report_sheets_final_cooke_rgb.pdf}
    \caption{Geometric defocus blur from Hendrycks et al. vs. astigmatic lens model.}
    \label{fig:my_label}
\end{figure}
%
\begin{figure}[h]
    \centering
    \includegraphics[page=25,width=\linewidth]{figures/matching/report_sheets_final_cooke_rgb.pdf}
    \caption{Geometric defocus blur from Hendrycks et al. vs. coma aberration, severity 5.}
    \label{fig:my_label}
\end{figure}
%
\
\begin{figure}[h]
    \centering
    \includegraphics[width=\linewidth]{figures/eval_rg/report_acc_over_severitysplit_corruptions_mode_trefoilrefvar_defocus_blur.pdf}
    \caption{Relative accuracy for trefoil and defocus blur.}
    \label{fig:my_label}
\end{figure}


\newpage

\begin{figure}[h]
    \centering
    \includegraphics[page=39,width=\linewidth]{figures/matching/report_sheets_final_cooke_rgb.pdf}
    \caption{Geometric defocus blur from Hendrycks et al. vs. trefoil aberration.}
    \label{fig:my_label}
\end{figure}



\begin{figure}[h]
    \centering
    \includegraphics[width=\linewidth]{figures/eval_rg/report_acc_over_severitysplit_corruptions_refvar_sub_defocus_blur.pdf}
    \caption{Difference in accuracy compared to defocus blur. Color groups represent the different corruptions.}
    \label{fig:my_label}
\end{figure}
\fi



\iffalse
\begin{figure}
    \centering    
    \includegraphics[width=\linewidth]{figures/imagenet100/eval_rgb/report_rank_baseline_trefoil_severity5.pdf}
    \caption{Ranking comparison of baseline (here: astigmatism) and coma for severity 5. The DNNs with pre-computed augmentation on ImageNet-100 achieve better results than the ones without any augmentation during training.}
    \label{fig:my_label}
\end{figure}
\fi


%%%%%%%%%%%%%%%%%%%%%%%%%%%%%%%%%%%%%%%%%%%%%%%%%%%%%%%%%%
%%%%%%%%%%%%%%%%%% (intended for) %%%%%%%%%%%%%%%%%%%%%%%%%%
%%%%%%%%%%%%%%%%%%% supplementary %%%%%%%%%%%%%%%%%%%%%%%%
%%%%%%%%%%%%%%%%%  submission due 15th of march %%%%%%%%%%%%%
%%%%%%%%%%%%%%%%%%%%%%%%%%%%%%%%%%%%%%%%%%%%%%%%%%%%%%%%%%%%
% https://iccv2023.thecvf.com/submission.guidelines-361600-2-20-16.php 
\iffalse
\newpage
\section{ImageNet100 and ImageNet100-C}
\label{app:imagenet100_and_c}
\begin{figure}[h]
 \begin{subfigure}{\linewidth}
    \centering
    \includegraphics[width=\linewidth]{figures/imagenet100-c/eval_rgb/report_acc_over_severitysplit_corruptions_highlight_resnet101_sgd_clean_resnet101_sgd_opticsaugment.pdf}
    \caption{ResNet101 clean (red) vs. OpticsAugment (blue).}
    \label{fig:common2d_modes_opticsaugment_resnet101}
\end{subfigure}
 \begin{subfigure}{\linewidth}
    \centering
    \includegraphics[width=\linewidth]{figures/imagenet100-c/eval_rgb/report_acc_over_severitysplit_corruptions_highlight_efficientnet_b0_sgd_clean_efficientnet_b0_sgd_opticsaugment.pdf}
    \caption{EfficientNet clean (red) vs. OpticsAugment (blue).}
    \label{fig:common2d_modes_opticsaugment_efficientnet}
\end{subfigure}
 \begin{subfigure}{\linewidth}
    \centering
    \includegraphics[width=\linewidth]{figures/imagenet100-c/eval_rgb/report_acc_over_severitysplit_corruptions_highlight_mobilenet_v3_large__clean_mobilenet_v3_large__opticsaugment.pdf}
    \caption{MobileNet\_v3 clean (red) vs. OpticsAugment (blue).}
    \label{fig:common2d_modes_opticsaugment_mobilenet}
\end{subfigure}\begin{subfigure}{\linewidth}
    \centering
    \includegraphics[trim=2cm 8.3cm 0.5cm 0cm,clip,width=0.9\linewidth]{figures/imagenet100-c/eval_rgb/labels_only_severity_split.pdf}
    \caption{Selected 2D common corruptions.}
\end{subfigure}
    \caption{Evaluation of 2D common corruptions for the DNNs trained on ImageNet-100 with and without OpticsAugment. }
    \label{fig:common2d_modes_appendix}
\end{figure}


%%%%%%%%%%%%%%%%% ResNet101 %%%%%%%%%%%%%%%%%%%%%%%%%%%%%%%
\begin{figure}[h]
 \begin{subfigure}{\linewidth}
    \centering
    \includegraphics[width=\linewidth]{figures/imagenet100-c/eval_rgb/report_acc_over_severitysplit_corruptions_clean_resnet101.pdf}
    \caption{Highlighted: ResNet101 clean (no augmentation)}
    \label{fig:common2d_modes_clean}
\end{subfigure}
 \begin{subfigure}{\linewidth}
    \centering
    \includegraphics[width=\linewidth]{figures/imagenet100-c/eval_rgb/report_acc_over_severitysplit_corruptions_opticsaugment_resnet101.pdf}
    \caption{Highlighted: ResNet101 clean + OpticsAugment}
    \label{fig:common2d_modes_opticsaugment}
\end{subfigure}
 \begin{subfigure}{\linewidth}
    \centering
    \includegraphics[trim=2cm 8.3cm 0.5cm 0cm,clip,width=0.9\linewidth]{figures/imagenet100-c/eval_rgb/labels_only_severity_split.pdf}
    \caption{2D common corruptions evaluated in Fig.~\ref{fig:common2d_modes_clean} and Fig.~\ref{fig:common2d_modes_opticsaugment}.}
\end{subfigure}
    \caption{Evaluation of 2D common corruptions for the DNNs trained on ImageNet-100 with and without OpticsAugment. }
    \label{fig:common2d_modes}
\end{figure}


%%%%%%%%%%%%%%%%% DenseNet161 %%%%%%%%%%%%%%%%%%%%%%%%%%%%%%%
\begin{figure}[h]
 \begin{subfigure}{\linewidth}
    \centering
    \includegraphics[width=\linewidth]{figures/imagenet100-c/eval_rgb/report_acc_over_severitysplit_corruptions_clean_\network.pdf}
    \caption{Highlighted: DenseNet clean (no augmentation)}
    \label{fig:common2d_modes_clean}
\end{subfigure}
 \begin{subfigure}{\linewidth}
    \centering
    \includegraphics[width=\linewidth]{figures/imagenet100-c/eval_rgb/report_acc_over_severitysplit_corruptions_opticsaugment_\network.pdf}
    \caption{Highlighted: DenseNet clean + OpticsAugment}
    \label{fig:common2d_modes_opticsaugment}
\end{subfigure}
 \begin{subfigure}{\linewidth}
    \centering
    \includegraphics[trim=2cm 8.3cm 0.5cm 0cm,clip,width=0.9\linewidth]{figures/imagenet100-c/eval_rgb/labels_only_severity_split.pdf}
    \caption{2D common corruptions evaluated in Fig.~\ref{fig:common2d_modes_clean} and Fig.~\ref{fig:common2d_modes_opticsaugment}.}
\end{subfigure}
    \caption{Evaluation of 2D common corruptions for the DNNs trained on ImageNet-100 with and without OpticsAugment. }
    \label{fig:common2d_modes}
\end{figure}

%%%%%%%%%%%%%%%%% EfficientNet b0 %%%%%%%%%%%%%%%%%%%%%%%%%%%%%%%
\begin{figure}[h]
 \begin{subfigure}{\linewidth}
    \centering
    \includegraphics[width=\linewidth]{figures/imagenet100-c/eval_rgb/report_acc_over_severitysplit_corruptions_clean_efficientnet.pdf}
    \caption{Highlighted: EfficientNet clean (no augmentation)}
    \label{fig:common2d_modes_clean}
\end{subfigure}
 \begin{subfigure}{\linewidth}
    \centering
    \includegraphics[width=\linewidth]{figures/imagenet100-c/eval_rgb/report_acc_over_severitysplit_corruptions_opticsaugment_efficientnet.pdf}
    \caption{Highlighted: EfficentNet clean + OpticsAugment}
    \label{fig:common2d_modes_opticsaugment}
\end{subfigure}
 \begin{subfigure}{\linewidth}
    \centering
    \includegraphics[trim=2cm 8.3cm 0.5cm 0cm,clip,width=0.9\linewidth]{figures/imagenet100-c/eval_rgb/labels_only_severity_split.pdf}
    \caption{2D common corruptions evaluated in Fig.~\ref{fig:common2d_modes_clean} and Fig.~\ref{fig:common2d_modes_opticsaugment}.}
\end{subfigure}
    \caption{Evaluation of 2D common corruptions for the DNNs trained on ImageNet-100 with and without OpticsAugment. }
    \label{fig:common2d_modes}
\end{figure}

%%%%%%%%%%%%%%%%% ResNeXt50 %%%%%%%%%%%%%%%%%%%%%%%%%%%%%%%
\begin{figure}[h]
 \begin{subfigure}{\linewidth}
    \centering
    \includegraphics[width=\linewidth]{figures/imagenet100-c/eval_rgb/report_acc_over_severitysplit_corruptions_clean_resnext50.pdf}
    \caption{Highlighted: ResNext50 clean (no augmentation)}
    \label{fig:common2d_modes_clean}
\end{subfigure}
 \begin{subfigure}{\linewidth}
    \centering
    \includegraphics[width=\linewidth]{figures/imagenet100-c/eval_rgb/report_acc_over_severitysplit_corruptions_opticsaugment_resnext50.pdf}
    \caption{Highlighted: ResNext50 clean + OpticsAugment}
    \label{fig:common2d_modes_opticsaugment}
\end{subfigure}
 \begin{subfigure}{\linewidth}
    \centering
    \includegraphics[trim=2cm 8.3cm 0.5cm 0cm,clip,width=0.9\linewidth]{figures/imagenet100-c/eval_rgb/labels_only_severity_split.pdf}
    \caption{2D common corruptions evaluated in Fig.~\ref{fig:common2d_modes_clean} and Fig.~\ref{fig:common2d_modes_opticsaugment}.}
\end{subfigure}
    \caption{Evaluation of 2D common corruptions for the DNNs trained on ImageNet-100 with and without OpticsAugment. }
    \label{fig:common2d_modes}
\end{figure}


%%%%%%%%%%%%%%%%% MobileNet %%%%%%%%%%%%%%%%%%%%%%%%%%%%%%%
\begin{figure}[h]
 \begin{subfigure}{\linewidth}
    \centering
    \includegraphics[width=\linewidth]{figures/imagenet100-c/eval_rgb/report_acc_over_severitysplit_corruptions_clean_mobilenet.pdf}
    \caption{Highlighted: MobileNet clean (no augmentation)}
    \label{fig:common2d_modes_clean}
\end{subfigure}
 \begin{subfigure}{\linewidth}
    \centering
    \includegraphics[width=\linewidth]{figures/imagenet100-c/eval_rgb/report_acc_over_severitysplit_corruptions_opticsaugment_mobilenet.pdf}
    \caption{Highlighted: MobileNet clean + OpticsAugment}
    \label{fig:common2d_modes_opticsaugment}
\end{subfigure}
 \begin{subfigure}{\linewidth}
    \centering
    \includegraphics[trim=2cm 8.3cm 0.5cm 0cm,clip,width=0.9\linewidth]{figures/imagenet100-c/eval_rgb/labels_only_severity_split.pdf}
    \caption{2D common corruptions evaluated in Fig.~\ref{fig:common2d_modes_clean} and Fig.~\ref{fig:common2d_modes_opticsaugment}.}
\end{subfigure}
    \caption{Evaluation of 2D common corruptions for the DNNs trained on ImageNet-100 with and without OpticsAugment. }
    \label{fig:common2d_modes}
\end{figure}
\fi


\iffalse
\begin{table}[h]
    \caption{Selection of pretrained models from pytorch vision and (RobustBench model zoos) with corresponding number of trainable parameters. The selected neural networks from RobustBench use a ResNet50.}
    \label{}    
    \centering
    \begin{tabular}{l l l}
    Architecture & Variants &  Parameter $[\times 10^6]$\\
    (AlexNet) &  & \\
    ConvNeXt & (tiny,small,base,large) & \\
    DenseNet & (161,169,201) & \\
    EfficientNet & (b0-b7) &\\
    Inception\_v3 & & \\
    MobileNet & (2,3) & \\ 
    MnasNet &  (0.5,0.75,1.0,1.3) & \\
    ShuffleNet &  &\\
    SqueezeNet & (1\_0,1\_1) &\\
    RegNetX & (400mf,800mf,1\_gf,3\_2gf,8\_gf) &\\
    RegNetY & (400mf,800mf,1\_gf,3\_2gf,8\_gf) &\\
    ResNet     &  (50,101,152) & \\
    ResNet (wide) &  (50,101) & \\
    ResNeXt     &  (50,101) & \\
    VGG &  (11,13,16,19) & \\
    \end{tabular}
    \centering
\end{table}
\fi

\iffalse 
% model list 
['alexnet', 'resnet18', 'resnet34', 'resnet50', 'resnet101', 'resnet152', 'resnext50_32x4d', 'resnext101_32x8d', 'wide_resnet50_2', 'wide_resnet101_2', 'vgg11', 'vgg11_bn', 'vgg13', 'vgg13_bn', 'vgg16', 'vgg16_bn', 'vgg19_bn', 'vgg19', 'squeezenet1_0', 'squeezenet1_1', 'inception_v3', 'densenet121', 'densenet169', 'densenet201', 'densenet161', 'mobilenet_v2', 'mobilenet_v3_large', 'mobilenet_v3_small', 'mnasnet0_5', 'mnasnet0_75', 'mnasnet1_0', 'mnasnet1_3', 'shufflenet_v2_x0_5', 'shufflenet_v2_x1_0', 'shufflenet_v2_x1_5', 'shufflenet_v2_x2_0', 'efficientnet_b0', 'efficientnet_b1', 'efficientnet_b2', 'efficientnet_b3', 'efficientnet_b4', 'efficientnet_b5', 'efficientnet_b6', 'efficientnet_b7',  'regnet_x_400mf', 'regnet_x_800mf', 'regnet_x_1_6gf', 'regnet_x_3_2gf', 'regnet_x_8gf', 'regnet_x_16gf', 'regnet_x_32gf', 
'regnet_y_800mf', 'regnet_y_1_6gf', 'regnet_y_3_2gf', 'regnet_y_8gf', 'regnet_y_16gf', 'regnet_y_32gf', 'vit_b_16','vit_b_32','vit_l_16','vit_l_32',\
'convnext_tiny','convnext_small','convnext_base','convnext_large']
\fi

\iffalse
\begin{figure}[h]
    \centering
    \includegraphics[width=\linewidth]{figures/eval_rgb/report_acc_over_severitysplit_corruptions.pdf}
    \caption{Accuracy for the different severities. Colors refer to the different corruptions from left to the right. The red diamonds show the accuracy for ConvNeXt\_base.}
    \label{fig:acc_vs_severity}
\end{figure}
\fi
